# Supplementary material for: Stresslets induced by active swimmers
Source: arXiv:1609.03275 ancillary file (2019-02-14)
Supplement: Supplementary file 1 [file SI.pdf]

# Supplemental Information to "Stresslets induced by active swimmers"

Eric Lauga[1,*] and Sebastien Michelin[2,†]
[1] Department of Applied Mathematics and Theoretical Physics, University of Cambridge, CB3 0WA, United Kingdom.
[2] LadHyX – Département de Mécanique, Ecole Polytechnique – CNRS, 91128 Palaiseau, France.
(Dated: September 12, 2016)

## I. DIRECT CALCULATION OF THE STRESSLET OF A SQUIRMING SPHERE

In the reference frame of a translating force-free sphere, the velocity field generated by an axisymmetric tangential slip flow at the sphere's boundary $\mathbf{u}(r=a) = u_s(\zeta)\mathbf{e}_\theta$ can be written as a superposition of squirming modes [1, 2]. With $\zeta = \cos\theta$ in spherical polar coordinates,

$$\mathbf{u} = \sum_{n=1}^{\infty} \frac{(2n+1)\alpha_n}{n(n+1)} \left[ \frac{\psi_n(r)}{r^2} L_n(\zeta)\mathbf{e}_r - \sqrt{1-\zeta^2} L_n'(\zeta) \frac{\psi_n'(r)}{r} \mathbf{e}_\theta \right], \tag{1}$$

with

$$\psi_1(r) = \frac{a^3 - r^3}{3r}, \quad \psi_{n\geq 2}(r) = \frac{1}{2}\left(\frac{a^n}{r^{n-2}} - \frac{a^{n+2}}{r^n}\right), \tag{2}$$

$$\alpha_n(t) = \frac{1}{2}\int_{-1}^{1} u_s(\zeta)\sqrt{1-\zeta^2} L_n'(\zeta)\mathrm{d}\zeta. \tag{3}$$

The traction on the boundary of the squirmer ($r = a$) can also be computed explicitly as

$$\boldsymbol{\sigma}\cdot\mathbf{n} = -\frac{3\mu\alpha_1}{a}(2\zeta\mathbf{e}_r + \sqrt{1-\zeta^2}\mathbf{e}_\theta) - \frac{\mu}{a}\sum_{n=2}^{\infty}\frac{(2n+1)\alpha_n}{n(n+1)}\left[3nL_n(\zeta)\mathbf{e}_r + (2n+1)\sqrt{1-\zeta^2}L_n'(\zeta)\mathbf{e}_\theta\right]. \tag{4}$$

Using the definition of the stresslet, Eq. (1) in the main article, with $\mathbf{n} = \mathbf{e}_r$ and $\mathbf{x} = a\mathbf{e}_r$ on the boundary

$$\begin{aligned}
\mathbf{S} =& 2\pi\mu a^2 \int_{-1}^{1} \left[ a\sigma_{rr}\langle \mathbf{e}_r\mathbf{e}_r\rangle_\phi + (a\sigma_{r\theta} - 2\mu u_\theta)\frac{\langle \mathbf{e}_r\mathbf{e}_\theta\rangle_\phi + \langle \mathbf{e}_\theta\mathbf{e}_r\rangle_\phi}{2}\right]\mathrm{d}\zeta \\
=& 2\pi\mu a^2\left(\mathbf{e}_z\mathbf{e}_z - \frac{\mathbf{I}}{3}\right)\int_{-1}^{1}\left[a\sigma_{rr}L_2(\zeta) - \frac{1}{2}(a\sigma_{r\theta} - 2\mu u_\theta)L_2'(\zeta)\sqrt{1-\zeta^2}\right]\mathrm{d}\zeta, \\
=& 10\pi a^2\mu\alpha_2\left(\mathbf{e}_z\mathbf{e}_z - \frac{\mathbf{I}}{3}\right),
\end{aligned} \tag{5}$$

or finally

$$\mathbf{S} = 15\pi a^2\mu\left(\mathbf{e}_z\mathbf{e}_z - \frac{\mathbf{I}}{3}\right)\int_{-1}^{1}\zeta\sqrt{1-\zeta^2}u_s(\zeta)\mathrm{d}\zeta. \tag{6}$$

## II. RECIPROCAL CALCULATION OF THE STRESSLET OF A SQUIRMING SPHERE

Using the results presented in this article, the stresslet of the squirming sphere can be directly computed from the slip velocity distribution provided one is able to find the tensor $\boldsymbol{\Sigma}$ such that the perturbation to the stress field

---

*Electronic address: e.lauga@damtp.cam.ac.uk
†Electronic address: sebastien.michelin@ladhyx.polytechnique.fr

introduced by a fixed rigid particle in a linear flow field $\mathbf{u} = -\mathbf{E}\cdot\mathbf{x}$ is defined as $\bar{\boldsymbol{\sigma}} = \boldsymbol{\Sigma} : \mathbf{E}$. For a given $\mathbf{E}$, the perturbation flow and pressure field are obtained [3] as

$$\bar{\mathbf{u}} = a^5 \frac{\mathbf{E}\cdot\mathbf{x}}{r^5} + \frac{5(\mathbf{x}\cdot\mathbf{E}\cdot\mathbf{x})\mathbf{x}}{2}\left(\frac{a^3}{r^5} - \frac{a^5}{r^7}\right), \tag{7}$$

$$\bar{p} = 5a^3\mu\frac{\mathbf{x}\cdot\mathbf{E}\cdot\mathbf{x}}{r^5}, \tag{8}$$

Taking the symmetric part of the gradient of the flow field, the stress tensor $\boldsymbol{\sigma} = -\bar{p}\mathbf{1} + \mu(\nabla\bar{\mathbf{u}} + \nabla\bar{\mathbf{u}}^T)$ is computed as

$$\bar{\boldsymbol{\sigma}} = \frac{2\mu a^5}{r^5}\mathbf{E} + \frac{5\mu a^3}{r^5}\left(\mathbf{x}(\mathbf{E}\cdot\mathbf{x}) + (\mathbf{E}\cdot\mathbf{x})\mathbf{x}\right) - \frac{5\mu a^5}{r^7}\left((\mathbf{x}\cdot\mathbf{E}\cdot\mathbf{x})\mathbf{I} + 2\mathbf{x}(\mathbf{E}\cdot\mathbf{x}) + 2(\mathbf{E}\cdot\mathbf{x})\mathbf{x}\right) + 5\mu(\mathbf{x}\cdot\mathbf{E}\cdot\mathbf{x})\mathbf{x}\mathbf{x}\left(\frac{7a^5}{r^9} - \frac{5a^3}{r^7}\right) \tag{9}$$

Therefore, from the definition of $\boldsymbol{\Sigma}$,

$$\begin{aligned}\Sigma_{klij} = {} & \frac{\mu a^5}{r^5}(\delta_{ik}\delta_{jl} + \delta_{jk}\delta_{il}) + \frac{5\mu a^3}{2r^5}(\delta_{il}x_jx_k + \delta_{ki}x_jx_l + \delta_{jl}x_ix_k + \delta_{kj}x_ix_l) \\ & - \frac{5\mu a^5}{r^7}(\delta_{kl}x_ix_j + \delta_{jl}x_kx_i + \delta_{il}x_jx_k + \delta_{jk}x_ix_l + \delta_{ik}x_jx_l) + 5\mu\left(\frac{7a^5}{r^9} - \frac{5a^3}{r^7}\right)x_ix_jx_kx_l,\end{aligned} \tag{10}$$

and on the sphere's surface

$$\Sigma_{klij} - \frac{1}{3}\Sigma_{klmm}\delta_{ij} - \mu\delta_{ik}\delta_{jl} - \mu\delta_{il}\delta_{jk} = -\frac{5}{2}\mu(\delta_{il}n_jn_k + \delta_{ik}n_jn_l + \delta_{jl}n_in_k + \delta_{jk}n_in_l + 2\delta_{kl}n_in_j - 4n_in_jn_kn_l) + \mu\delta_{kl}\delta_{ij}. \tag{11}$$

Then, applying the fundamental result of the main article, Eq. (7), the stresslet of a general spherical active particle is obtained as

$$\begin{aligned}S_{ij} = {} & \mu\iint_{\partial V} n_lu_k\left[-\frac{5}{2}(\delta_{il}n_jn_k + \delta_{ik}n_jn_l + \delta_{jl}n_in_k + \delta_{jk}n_in_l + 2\delta_{kl}n_in_j - 4n_in_jn_kn_l) + \delta_{kl}\delta_{ij}\right]\mathrm{d}A, \\ = {} & -\frac{5\mu}{2}\iint_{\partial V}(n_iu_j + n_ju_i)\mathrm{d}A.\end{aligned} \tag{12}$$

## III. DIRECT CALCULATION OF THE STRESSLET OF AN ACTIVE ROD

An active rod of length $L$ and orientation vector $\mathbf{p}$ is considered. The rod is slender enough so that resistive force theory can be used to determine the force density applied on the rod. First we note that the last terms in Eq. (1) of the main article disappear since

$$\iint_{\partial V} u_in_j\mathrm{d}A = \int_L u(s)\mathbf{p}_i\left(\int_{\partial V_R(s)} n_j\mathrm{d}A_R(s)\right)\mathrm{d}s \tag{13}$$

where $A_R(s)$ is the circle around the rod at section $s$. Clearly by symmetry the integral $\int_{\partial V_R(s)}\mathbf{n}\mathrm{d}A_R(s) = \mathbf{0}$ and thus these terms disappear. Calling $\mathbf{f}$ the force per unit length exerted on the swimming rod, the stresslet is given by

$$\mathbf{S} = \int_L\left[\frac{1}{2}(\mathbf{f}\mathbf{x} + \mathbf{x}\mathbf{f}) - \frac{1}{3}(\mathbf{f}\cdot\mathbf{x})\mathbf{I}\right]\mathrm{d}s. \tag{14}$$

To determine $\mathbf{f}$ we need to pay a closer look to the velocity distribution on the rod. We call $U\mathbf{p}$ the swimming speed and write the swimming gait as $u(s) = U_0\alpha(s)$ where $U_0$ is a characteristic velocity and $\alpha$ a dimensionless function characterising the distribution of velocity. The total velocity relative to the fluid at rest at infinity is

$$\mathbf{u} = U_0\alpha(s)\mathbf{p} + U\mathbf{p}, \tag{15}$$

resulting (resistive force theory) into a force per unit length $\mathbf{f}$ given by

$$\mathbf{f} = -\zeta_{||}[U_0\alpha(s) + U]\mathbf{p}, \tag{16}$$

where $\zeta_\parallel$ is the local tangential drag coefficient along the rod. Inertia is negligible and the rod is force-free, therefore $\int \mathbf{f}\mathrm{d}s = \mathbf{0}$ and thus the swimming speed is given by

$$U = -U_0\langle\alpha\rangle, \tag{17}$$

where $\langle\alpha\rangle = (\int_L \alpha(s)\mathrm{d}s)/L$. The resulting force density is thus

$$\mathbf{f}(s) = -\zeta_\parallel U_0[\alpha(s) - \langle\alpha\rangle]\mathbf{p}. \tag{18}$$

From this result and using $\mathbf{x} = s\mathbf{p}$ and $\zeta_\parallel = \zeta_\perp/2$ with $\zeta_\perp$ the normal drag coefficient, the stresslet can be computed from Eq. (14) above:

$$\mathbf{S} = -\zeta_\parallel \int_L \left(U_0 s[\alpha(s) - \langle\alpha\rangle]\mathbf{pp} - \frac{1}{3}U_0 s[\alpha(s) - \langle\alpha\rangle]\mathbf{I}\right)\mathrm{d}s = -\frac{\zeta_\perp}{2}\left(U_0\int_L s[\alpha(s) - \langle\alpha\rangle]\mathrm{d}s\right)\left(\mathbf{pp} - \frac{1}{3}\mathbf{I}\right). \tag{19}$$

Defining $s$ in $[-L/2, L/2]$, this result is strictly equivalent to the reciprocal calculation presented in the main text, Eq. (17).

## IV. ELLIPSOID

### A. Spheroidal coordinates

We consider here a general axisymmetric ellipsoid of axis $\mathbf{e}_z$, and note $a$ (resp. $b$) the semi-axis along $\mathbf{e}_z$ (in the plane normal to $\mathbf{e}_z$). The ellipsoid is characterized by its surface are noted $\mathscr{S}$ and its aspect ratio $\xi = a/b$. $\xi \geq 1$ (resp. $\xi \leq 1$) corresponds to a prolate (resp. oblate) spheroid. Prolate (resp. oblate) spheroidal coordinates $(\tau, \zeta, \phi)$ are defined such that $z = k\tau\zeta$ and $(x, y) = k\sqrt{(\tau^2 - 1)(1 - \zeta^2)}(\cos\phi, \sin\phi)$ (resp. $(x, y) = k\sqrt{(\tau^2 + 1)(1 - \zeta^2)}(\cos\phi, \sin\phi)$). $k$ is a positive scaling constant that relates the aspect ratio $\xi$ and the surface area of the ellipsoid (see main text). The unit vectors and scale factors can be expressed for both oblate and prolate spheroids, at the surface of the ellipsoid *only* (i.e. for $\tau = \xi/\sqrt{|\xi^2 - 1|}$), as

$$h_\tau = k\sqrt{\zeta^2 + \xi^2(1 - \zeta^2)}, \quad \mathbf{e}_\tau = \frac{\xi\sqrt{1 - \zeta^2}(\mathbf{e}_\phi \times \mathbf{e}_z) + \zeta\mathbf{e}_z}{\sqrt{\zeta^2 + \xi^2(1 - \zeta^2)}} \tag{20}$$

$$h_\zeta = k\sqrt{\frac{\zeta^2 + \xi^2(1 - \zeta^2)}{(1 - \zeta^2)|\xi^2 - 1|}}, \quad \mathbf{e}_\zeta = \frac{-\zeta(\mathbf{e}_\phi \times \mathbf{e}_z) + \xi\sqrt{1 - \zeta^2}\mathbf{e}_z}{\sqrt{\zeta^2 + \xi^2(1 - \zeta^2)}} \tag{21}$$

$$h_\phi = k\sqrt{\frac{1 - \zeta^2}{|\xi^2 - 1|}}, \quad \mathbf{e}_\phi = -\sin\phi\,\mathbf{e}_x + \cos\phi\,\mathbf{e}_y. \tag{22}$$

The area of the ellipsoid's surface can be expressed as

$$\mathscr{S} = \frac{2\pi k^2}{|\xi^2 - 1|}\left[1 + \frac{\xi^2}{\sqrt{\xi^2 - 1}}\cos^{-1}\left(\frac{1}{\xi}\right)\right]. \tag{23}$$

### B. Jeffery's solution

Following [4], the solution of Stokes' equations that decay at infinity and satisfies $\bar{\mathbf{u}} = E(\mathbf{e}_z\mathbf{e}_z - \mathbf{1}/3)\cdot\mathbf{x}$ at the spheroid's boundary is obtained as

$$\bar{\mathbf{u}} = \nabla \times (\mathbf{B}\cdot\boldsymbol{\chi}) + [(\mathbf{A}\cdot\mathbf{x})\cdot\nabla]\,\nabla\varphi - \mathbf{A}\cdot\nabla\varphi, \tag{24}$$

with

$$\varphi(\mathbf{x}) = \int_{\lambda(\mathbf{x})}^{\infty} \left[\frac{z^2}{a^2+u} + \frac{x^2+y^2}{b^2+u}\right] \frac{\mathrm{d}u}{(b^2+u)\sqrt{a^2+u}}, \tag{25}$$

$$\boldsymbol{\chi}(\mathbf{x}) = (xz\mathbf{e}_y + yz\mathbf{e}_x) \int_{\lambda(\mathbf{x})}^{\infty} \frac{\mathrm{d}u}{(a^2+u)^{3/2}(b^2+u)^2}, \tag{26}$$

$$\mathbf{A} = -\frac{b^3}{6}\frac{\mathbf{E}}{F(\xi)}, \quad F(\xi) = \xi \int_0^{\infty} \frac{u\mathrm{d}u}{(1+u)^2(\xi^2+u)^{3/2}}, \tag{27}$$

$$\mathbf{B} = -\frac{b^3(2a^2+b^2)E}{9F(\xi)} \left(-\mathbf{e}_x\mathbf{e}_x + \mathbf{e}_y\mathbf{e}_y\right), \tag{28}$$

and $\lambda(\mathbf{x})$ is the positive root of

$$\frac{z^2}{a^2+\lambda} + \frac{x^2+y^2}{b^2+\lambda} = 1. \tag{29}$$

The force applied on the spheroid's boundary is then

$$\bar{\boldsymbol{\sigma}} \cdot \mathbf{n} = 2\mu \left[\frac{2G(\xi)}{9F(\xi)} E\mathbf{1} + \left(1 - \frac{2}{3F(\xi)}\right)\mathbf{E}\right] \cdot \mathbf{n}, \tag{30}$$

with

$$G(\xi) = \int_0^{\infty} \frac{\xi(1-\xi^2)\mathrm{d}u}{(1+u)^2(\xi^2+u)^{3/2}}. \tag{31}$$

### C. Reciprocal calculation of the stresslet of an active ellipsoid

Considering now an active spheroid prescribing a slip velocity at its boundary, the approach followed to derive Eq. (6) in the main text can be adapted to the present axisymmetric setting in order to derive the traction part of the resulting stresslet as

$$\iint_{\partial V} \frac{1}{2}\left[(\mathbf{x}(\boldsymbol{\sigma}\cdot\mathbf{n}) + (\boldsymbol{\sigma}\cdot\mathbf{n})\mathbf{x}) - \frac{\mathbf{x}\cdot\boldsymbol{\sigma}\cdot\mathbf{n}}{3}\mathbf{1}\right]\mathrm{d}S = \mu\left(1 - \frac{2}{3F(\xi)}\right)\iint_{\partial V} (\mathbf{un}+\mathbf{nu})\mathrm{d}S, \tag{32}$$

and finally

$$\mathbf{S} = -\frac{2\mu}{3F(\xi)}\iint_{\partial V} (\mathbf{un}+\mathbf{nu})\mathrm{d}S. \tag{33}$$

### D. Finding the concentration distribution around an axisymmetric catalytic particle

The previous result can be used to determine the stresslet generated by an active autophoretic (or catalytic) particle of spheroidal shape whose surface properties are axisymmetric and characterized by a chemical activity (i.e. solute release rate) $\mathcal{A}(\zeta)$ and mobility $\mathcal{M}(\zeta)$. Writing $c$ the concentration of the solute, and neglecting advection, the solute dynamics is completely described by the following Laplace problem:

$$D\nabla^2 c = 0, \quad D\mathbf{e}_\tau \cdot \nabla c|_{\partial V} = -\mathcal{A}(\zeta), \quad c(\mathbf{x}\to\infty) = 0, \tag{34}$$

and the slip velocity imposed by the particle at its surface is computed as $\mathbf{u}_s = \mathcal{M}(\zeta)(\mathbf{1}-\mathbf{nn})\cdot\nabla c$.

Laplace's equation is separable in spheroidal polar coordinates:

$$\nabla^2 c = \frac{1}{k^2(\tau^2 \pm \zeta^2)}\left\{\frac{\partial}{\partial\tau}\left[(\tau^2 \pm 1)\frac{\partial c}{\partial\tau}\right] + \frac{\partial}{\partial\zeta}\left[(1-\zeta^2)\frac{\partial c}{\partial\zeta}\right]\right\}, \tag{35}$$

where $\pm$ corresponds to oblate and prolate spheroids, respectively. Its general solution is of the form

$$c = \sum_{n=0}^{\infty} c_n C_n(\tau) L_n(\zeta), \tag{36}$$

with $C_n(\tau) = Q_n(\tau)$ or $Q_n(\mathrm{i}\tau)$ for prolate and oblate spheroids, respectively, and $Q_n$ is the $n$-th Legendre function of second kind. Using $\mathbf{e}_\tau \cdot \nabla c = 1/h_\tau(\partial c/\partial \tau)$, the Neuman boundary condition for $c$ on the particle's surface can be projected along $L_n(\zeta)$ using the orthogonality of Legendre polynomials

$$\int_{-1}^{1} L_n(\zeta) L_p(\zeta) \mathrm{d}\zeta = \frac{2\delta_{np}}{2n+1}, \tag{37}$$

to obtain the concentration distribution

$$c(\tau, \zeta) = -\sum_{n=0}^{\infty} \frac{k(2n+1) C_n(\tau)}{2DC'_n(\tau_0)} \mathcal{I}_n(\xi) L_n(\zeta) \tag{38}$$

$$\mathcal{I}_n(\xi) = \int_{-1}^{1} \mathcal{A}(\zeta) \sqrt{\zeta^2 + \xi^2(1-\zeta^2)} L_n(\zeta) \mathrm{d}\zeta, \tag{39}$$

---


[1] H. Lamb. *Hydrodynamics.* Dover, New York, 6th edition, 1932.

[2] J. R. Blake. A spherical envelope approach to ciliary propulsion. *J. Fluid Mech.*, 46:199–208, 1971.

[3] L. G. Leal. *Advanced Transport Phenomena: Fluid Mechanics and Convective Transport Processes.* Cambridge University Press, Cambridge, UK, 2007.

[4] G. B. Jeffery. The motion of ellipsoidal particles immersed in a viscous fluid. *Proc. R. Soc. Lond. A*, 102:161–179, 1922.
